# Supplementary material for: Exploiting Instance-based Mixed Sampling via Auxiliary Source Domain Supervision for Domain-adaptive Action Detection
Source: arXiv:2209.15439 source file (2022-10-06)
Supplement: Supplementary file 2 [file TAB_sota_comparison_with_oracle.tex]

%\begin{table*}[t]
%\centering
%\begin{tabular}{c|cccccc|c}
%\toprule  
%Method&bend/bow&lie/sleep&run/jog&sit&stand&walk&mAP\\
%\midrule 
%Baseline w/o DA&33.66&54.82&56.82&\textbf{73.70}&\textbf{80.56}&\textbf{75.18}&62.46\\
%Rotation&25.53&58.86&55.05&72.42&79.84&68.49&60.03\\
%Clip-order&28.24&57.38&56.90&69.54&77.10&74.68&60.64\\
%\Gls{grl}&24.99&48.41&59.89&68.68&78.79&71.38&58.69\\
%\Gls{daaim} (w/ resize)&\textbf{33.79}&\textbf{59.27}&\textbf{62.16}&71.67&79.90&75.13&\textbf{63.65}\\
%\bottomrule 
%\end{tabular}
%\caption{\small{Kinetics $\to$ AVA: Evaluation results on AVA.}}
%\label{tab:kin2ava_target}
%\end{table*}

\begin{table*}[t]
\centering
% \captionsetup{font=footnotesize}
% \footnotesize
\caption{Evaluation results for \dalong with comparison to other \sotalong approaches without adding auxiliary domain. ``Baseline'' is trained on source and tested on target domain without any adaptation. Whereas ``Oracle'' is train and tested on target domain.}
\setlength{\tabcolsep}{4.5pt}
\resizebox{1.00\linewidth}{!}{
\begin{tabular}{lccccccc|cccc}
\toprule  
 & \multicolumn{7}{c}{\avakin $\to$ AVA} & \multicolumn{4}{c}{\avakin $\to$ \ihdtwo} \\
Method  & bend/bow & lie/sleep & run/jog & sit & stand & walk & mAP & touch & throw & take a photo & mAP\\
\midrule
Oracle model
&36.34&67.49&57.74&75.61&84.64&79.26&66.84&37.91&51.76&45.38&45.02\\
\midrule 
Source-only model
% ~\cite{feichtenhofer2019slowfast}
&33.66&54.82&56.82&\textbf{73.70}&\textbf{80.56}&\textbf{75.18}&62.46 &34.12&32.91&27.42&31.48\\
Rotation Prediction ~\cite{jing2018self} 
&25.53&58.86&55.05&72.42&79.84&68.49&60.03 &30.12&34.58&25.39&30.03\\
Clip-order Prediction ~\cite{xu2019self} 
&28.24&57.38&56.90&69.54&77.10&74.68&60.64 &28.28&32.30&29.93&30.17\\
GRL~\cite{agarwal2020unsupervised,chen2019temporal,ganin2015unsupervised} &24.99&48.41&59.89&68.68&78.79&71.38&58.69 &25.79&\textbf{39.71}&28.90&31.46 \\
\Gls{daaim} (ours) 
&\textbf{33.79}&\textbf{59.27}&\textbf{62.16}&71.67&79.90&75.13&\textbf{63.65}&\textbf{34.38}&35.65&\textbf{39.84}&\textbf{36.62}\\
\bottomrule 
\end{tabular}
}
\label{tab:sota_comparision_with_oracle}
\end{table*}
